# Supplementary material for: A probabilistic analysis on general probabilistic scheduling problems
Source: arXiv:2401.15677 source file (2024-01-28)
Supplement: Supplementary file 1 [file Appendix.tex]

\section{Appendix}
